# Supplementary material for: FAN: Focused Attention Networks
Source: arXiv:1905.11498 source file (2019-10-03)
Supplement: Supplementary file 1 [file appendix.tex]

% @inproceedings{belongie2007,
%   author    = {Andrew Rabinovich and
%               Andrea Vedaldi and
%               Carolina Galleguillos and
%               Eric Wiewiora and
%               Serge J. Belongie},
%   title     = {Objects in Context},
%   booktitle = {{IEEE} 11th International Conference on Computer Vision, {ICCV} 2007,
%               Rio de Janeiro, Brazil, October 14-20, 2007},
%   pages     = {1--8},
%   year      = {2007},
%   crossref  = {DBLP:conf/iccv/2007},
%   url       = {https://doi.org/10.1109/ICCV.2007.4408986},
%   doi       = {10.1109/ICCV.2007.4408986},
%   timestamp = {Wed, 14 Nov 2018 10:59:56 +0100},
%   biburl    = {https://dblp.org/rec/bib/conf/iccv/RabinovichVGWB07},
%   bibsource = {dblp computer science bibliography, https://dblp.org}
% }
